# Supplementary material for: Optical quantum memory on macroscopic coherence
Source: arXiv:2408.09991 source file (2024-08-19)
Supplement: Supplementary file 1 [file Moiseev_et_al_Supplement_Material.pdf]

# Supplemental material: Optical quantum memory on macroscopic coherence

S.A. Moiseev[1*] and K.I. Gerasimov[1],M.M. Minnegaliev[1], E.S. Moiseev [1]
[1]*Kazan Quantum Center, Kazan National Research Technical University n.a. A.N. Tupolev-KAI, 10 K. Marx St., 420111, Kazan, Russia*
(Dated: August 19, 2024)

## Photon echo quantum memory on a spin PLM-coherence

### A. Basic scheme and preparation of spin PLM-coherence

The basic four-level atomic levels of the proposed QM are shown in Fig.1, which contains two optical levels, each of which is split into 2 sublevels (the analysis carried out can also be applied to a three-level scheme with one optical level). Below we assume an absence of inhomogeneous broadening on spin transitions $|1\rangle \leftrightarrow |2\rangle$ and $|3\rangle \leftrightarrow |4\rangle$ where $\omega_{21}^j = \omega_{21}$ for the ground and $\omega_{43}^j = \omega_{43}$ for the excited optical sublevels. At the same time we take into account inhomogeneous broadening on the optical transition $|1\rangle \leftrightarrow |3\rangle$ described by the normalized formfactor $G(\Delta/\Delta_{in})$ with a linewidth $\Delta_{in}$ and similar inhomogeneous broadening on $|2\rangle \leftrightarrow |4\rangle$ optical transition. This level scheme is often used in experiments with

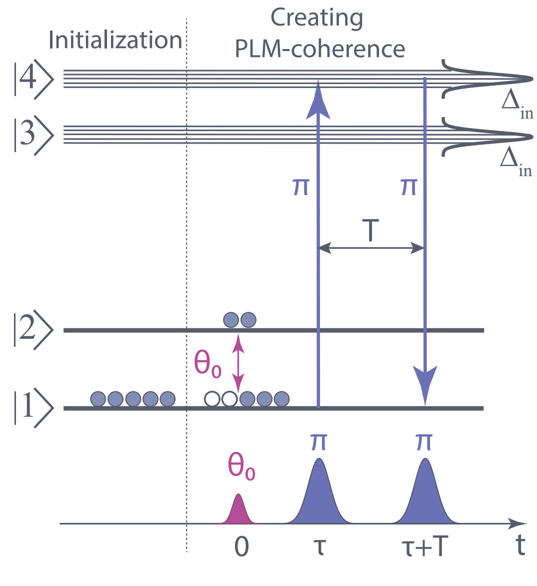


FIG. 1. Four atomic levels of the QM with PLM-coherence; RF pulse with pulse area $\theta_0$ (red arrow) creating spin coherence, two laser $\pi$-pulses (blue arrows). Many lines in the states $|3\rangle$, $|4\rangle$ indicate the presence of inhomogeneous broadening ($\Delta_{in}$) at the optical transitions.

rare earth ions, for example, with praseodymium ions in $Y_2SiO_5$ crystal [1, 2]. The Hamiltonian of the considered system of atoms has the form

$$\hat{H}_a = \hbar \sum_{j=1}^{N} \{(\Delta_j + \omega_{41})\hat{P}_{44}^j + (\Delta_j + \omega_{31})\hat{P}_{33}^j + \omega_{21}\hat{P}_{22}^j\}, \quad (1)$$

where $\hat{P}_{mn}^j = |n\rangle_{jj}\langle m|$, $N$ is a total number of atoms, $\hbar$ is reduced Planck's constant. Suppose that all atoms are initially prepared at the first sublevel 1, i.e. $|\Psi_a\rangle_{in} = \prod_{j=1}^{N} |1_j\rangle$, which is usually realized experimentally by selective laser pumping of the long lived sublevels 1 and 2, which also ensures a long lifetime of the quantum coherence $T_{2,s}$ at the spin transition $|1\rangle \leftrightarrow |2\rangle$, as it is implied in the further consideration.

At the next stage, we prepare a spin coherence on the transition the $|1\rangle \leftrightarrow |2\rangle$ by applying a resonant short intense radiofrequency (RF) pulse with a pulse area $\theta_0$. As a result, the quantum state of atoms takes the form:

$$|\Psi_a\rangle_1 = \hat{U}_{rf}(\theta_0, \varphi_0)\, |\Psi_a\rangle_{in}\,, \quad (2)$$

where $|\Psi_a\rangle_m = \prod_{j=1}^{N} \otimes |\psi_{a,m}\rangle_j$,

$$|\psi_{a,1}\rangle_j = \cos\left(\frac{\theta_0}{2}\right)|1_j\rangle - ie^{i\varphi_0^j}\sin\left(\frac{\theta_0}{2}\right)|2_j\rangle\,, \quad (3)$$

where $\varphi_0^j = \varphi_0 + i\mathbf{k}_0\mathbf{r}_j$ and $\mathbf{r}_j$ are phase and spatial coordinate of j-th atom, $\varphi_0$ and $\mathbf{k}_0$ are the phase and wave vector of the RF pulse.

The state (2) corresponds to the excitation of macroscopic spin coherence

$$\langle \hat{P}_{12}^j \rangle = \langle \psi_{a,1}|_j\, \hat{P}_{12}^j\, |\psi_{a,1}\rangle_j = -\frac{i}{2}\sin\theta_0 e^{i(\varphi_0 + i\mathbf{k}_0\mathbf{r}_j)}. \quad (4)$$

After a small time delay $\tau \ll T_{2,s}$ we launch a sequence of two laser pulses propagating along $\mathbf{k}_1$ and $\mathbf{k}_2$ directions with a time delay between them $T \gg \Delta_{in}$. We assume that the duration of these pulses is much shorter than the duration of the optical signal pulses ($\delta t_{1,2} \ll \delta t_s$), therefore we will consider them infinitely short. The laser pulses are resonant to the optical transition $|1\rangle \leftrightarrow |4\rangle$ and have the same pulse area $\theta_1 = \theta_2 = \pi$ with the time delay $T$ less than the coherence time of the optical transition $T < T_{2,o}$ where usually $T_{2,o} \ll T_{2,s}$. As a result of the

* s.a.moiseev@kazanqc.org

action of two laser pulses, we obtain the following atomic quantum state at $t = \tau + T$:

$$|\Psi_a\rangle_2 = \hat{U}_{c,2}(\theta_2)\hat{T}(T)\hat{U}_{c,1}(\theta_1)\hat{T}(\tau)\,|\Psi_a\rangle_1\,, \qquad (5)$$

where

$$\begin{aligned} &|\psi_{a,2}\rangle_j = \\ &-\exp\{-i(\Delta_j+\omega_{41})T + i(\varphi_{1,2}+\mathbf{k}_{1,2}\mathbf{r}_j)\}\cos\left(\frac{\theta_0}{2}\right)|1_j\rangle \\ &-ie^{i\varphi_0^j}\exp\{-i\omega_{21}(\tau+T)\}\sin\left(\frac{\theta_0}{2}\right)|2_j\rangle\,, \end{aligned} \qquad (6)$$

where $\mathbf{k}_{1,2} = \mathbf{k}_1 - \mathbf{k}_2$, $\varphi_{1,2} = \varphi_1 - \varphi_2$, $\varphi_1$ and $\varphi_2$ are the phases of laser pulses.

As can be seen in Eq.(6), the free evolution of optical quantum coherence between the action of two optical pulses in the presence of an inhomogeneous broadening of the optical transition leads to the following spin coherence of $j$-th atom:

$$\begin{aligned} \langle \hat{P}_{12}^j(\tau+T)\rangle &= \langle\Psi_a|_2\,\hat{P}_{12}^j\,|\Psi_a\rangle_2 \\ &= i\frac{\sin(\theta_0)}{2}e^{i\Delta_j T}e^{i\phi+i(\mathbf{k}_0-\mathbf{k}_{1,2})\mathbf{r}_j}, \end{aligned} \qquad (7)$$

where $\phi = \varphi_0 - \varphi_{1,2} + \omega_{31}T - \omega_{21}\tau$.

An additional phase shift $\Delta_j T$ in the amplitude of the ground quantum state $|1_a\rangle_j$ lead to the fast dephasing of the macroscopic spin coherence when $\langle\hat{S}_{12}(\tau+T)\rangle \sim e^{-\Delta_{in}T} \cong 0$ for Lorentzian shape of inhomogeneous broadening $G(\Delta/\Delta_{in}) = \Delta_{in}/(\pi(\Delta^2+\Delta_{in}^2))$. We can use such inhomogeneous broadening if the spectral width of the signal pulse is small enough $\delta\omega_s \ll \Delta_{in}$, which is assumed below to simplify the analysis.

After preparing the spin PLM-coherence, we launch a weak signal light pulse.

### B. Signal pulse recording stage

The signal light pulse propagates along z-direction with time delay $t_0$ after the second control pulse (Fig.2). The time delay can be sufficiently large $t_0 - \tau - T \gg T_{1,a}$ since the lifetime of the spin quantum coherence $T_{2,s}$ can be much longer than the lifetime of the optical transition $T_{1,a}$ ($T_{2,s} \gg T_{1,a}$). We will describe the interaction of a weak signal pulse and a photon echo in the Heisenberg picture, taking $|\Psi_a(\tau+T)\rangle_2$ as the initial state of the atoms when a signal pulse is launched into the atomic medium with resonance to the optical transition $|2\rangle \leftrightarrow |3\rangle$ ($\omega_s = \omega_{32}$). We also assume that the initial quantum state of the signal pulse $|\psi_{in}(t\to-\infty)\rangle$ contains, on average, a number of photons, much less than the number of atoms in a QM cell. The Hamiltonian of the considered system of atoms and the radiation interacting with them takes the form:

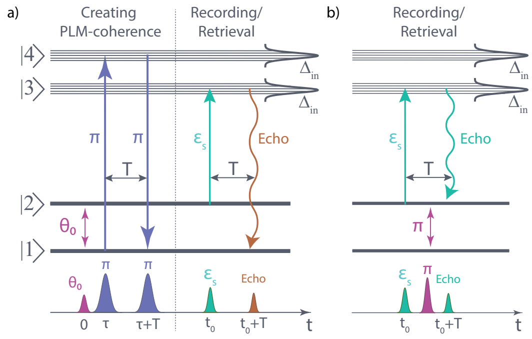


FIG. 2. Four atomic levels of the QM with PLM-coherence; RF pulse with pulse area $\theta_0$ (red arrow) creating spin coherence, two laser $\pi$-pulses (blue arrows), signal pulse (green arrow), echo pulse (yellow wavy arrow). Many lines in the states $|3\rangle$, $|4\rangle$ indicate the presence of inhomogeneous broadening at the optical transitions.

$$\hat{H}_{a+f} = \hat{H}_a + \hat{H}_f + \hat{V}_{int}, \qquad (8)$$

where $\hat{H}_f = \hbar\int dk\omega_k\hat{a}^\dagger(k)\hat{a}(k)$ , $\hat{V}_{int} = \hbar\sum_j^N g_s\hat{P}_{32}^j\int dk\hat{a}(k)e^{ikz_j} + H.C.$ are the Hamiltonians of radiation and its resonant interaction with atoms in dipole and rotating wave approximations; $g_s = E_0\langle\mathbf{d}_{23}\cdot\mathbf{e}\rangle/\hbar$ being a single photon Rabi-frequency, $\mathbf{e}$ is a polarization vector of the light field, $E_0 \cong (\frac{\hbar\omega_0}{2\varepsilon_0\varepsilon(\omega_0)S})^{1/2}$, $S$ is the cross-section of the light beam, $\varepsilon_0$ is the electric permittivity of vacuum, respectively [3].

Below we introduce slowly varying operators of signal field $\hat{b}_s(z,t)$ and atomic coherences $\hat{S}_{nm}^j$

$$\hat{b}_s(t,z) = e^{i\omega_s t - ik_s z}\hat{a}_s(t,z), \qquad (9)$$
$$\hat{S}_{23}^j(t) = e^{i\omega_s t - ik_s z}\hat{P}_{23}^j(t), \qquad (10)$$
$$\hat{S}_{13}^j(t) = e^{i\omega_{31} t - ik_s z}\hat{P}_{13}^j(t), \qquad (11)$$
$$\hat{S}_{12}^j(t) = e^{i\omega_{21} t}\hat{P}_{12}^j(t), \qquad (12)$$

where $[\hat{b}_s(t,z),\hat{b}_s^\dagger(t,z')] = 2\pi\delta(z-z')$, $\hat{a}_s(t,z) = \int dk\hat{a}(k,t)e^{ikz}$ with initial atomic parameters at $t = \tau + T$, determined by the state (5), (6) and (7): where $\langle\hat{S}_{12}^j(t>\tau+T)\rangle = \langle\hat{P}_{12}^j(\tau+T)\rangle$, $\langle\hat{S}_{13}^j\rangle = \langle\hat{S}_{23}^j\rangle = \langle\hat{S}_{33}^j\rangle = 0$, $\langle\hat{S}_{11}^j\rangle = \cos^2(\theta_0/2)$, $\langle\hat{S}_{22}^j\rangle = \sin^2(\theta_0/2)$.

Using Eqs. (1), (8) we obtain the following Heisenberg equations:

$$\left(\frac{\partial}{\partial t}+v_g\frac{\partial}{\partial z}\right)\hat{b}_s(z,t)=-2\pi i\sum_{j=1}^{N}g_s\hat{S}^j_{23}(t)\delta(z-z_j), \tag{13}$$

$$\frac{\partial\hat{S}^j_{23}(t)}{\partial t}=-i\Delta_j\hat{S}^j_{23}(t)-ig_s\hat{b}_s(z_j,t)\big[\hat{S}^j_{22}(t)-\hat{S}^j_{33}(t)\big], \tag{14}$$

$$\frac{\partial\hat{S}^j_{13}(t)}{\partial t}=-i\Delta_j\hat{S}^j_{13}(t)-ig_s\hat{b}_s(z_j,t)\hat{S}_{12}(t), \tag{15}$$

$$\frac{\partial\hat{S}^j_{12}(t)}{\partial t}=-ig^*_s\hat{b}^\dagger_s(z_j,t)\hat{S}_{13}(t), \tag{16}$$

where for further convenience the summation of an arbitrary function $F(z_j,\Delta_j,t)$ over the atoms in Eq.(13) may be approximated in continuous limit as an integration

$$\sum_{j=1}^{N}\hat{F}(z_j,\Delta_j,t)\delta(z-z_j)=\rho\int d\Delta G(\Delta/\Delta_{in})\hat{F}(z,\Delta,t), \tag{17}$$

where $\rho=\frac{N}{L}$ is a linear atomic density, L is a spatial size of the atomic medium.

In Eqs. (13)-(16) we take into account that the signal pulse is very weak, without significantly affecting the initial population of the atomic levels so $\langle\hat{S}^j_{22}(t)\rangle-\langle\hat{S}^j_{33}(t)\rangle\cong\langle\hat{S}^j_{22}(t)\rangle$ in Eq.(14). According to Eqs.(15), (16) the weak signal pulse negligibly effects on the spin coherence $S^j_{12}$ (only in the second order by interaction with weak signal field). Therefore, we can replace the operators $S^j_{22}(t)$ and $S^j_{12}(t)$ in Eqs. (14),(15) by their values before interaction with a signal light pulse ( at $t=t_s$) and to ignore an evolution of the prepared spin coherence $S^j_{12}(t)$ during the interaction with the signal pulse.

At the beginning, we will write down the formal solutions of the optical coherences $S^j_{23}(t)$, $S^j_{13}(t)$.

$$\hat{S}^j_{m3}(t)=e^{-i\Delta_j(t-\tau-T)}\hat{S}^j_{m3}(\tau+T)+\delta\hat{S}^j_{m3}(t), \tag{18}$$

where is the excited coherence

$$\delta\hat{S}^j_{m3}(t)=-ig_se^{-i\Delta_j(t-t_s)}\hat{S}^j_{m2}(\tau+T)\cdot \int_{\tau+T}^{t}dt'e^{-i\Delta_j(t'-t_s)}\hat{b}_s(t',z_j). \tag{19}$$

Although the evolution of signal field $\hat{b}_s(t,z)$ is coupled with macroscopic optical coherence $\langle\hat{S}_{23}\rangle$ by Eq. (13), (17), the effect of the signal field also leads, due to the presence of spin coherence $\hat{S}^j_{12}(t)$, to the appearance of atomic coherence $\hat{S}^j_{13}$ in Eq. (19) at the adjacent atomic transition. However, the excited collective macroscopic coherence $\langle\hat{S}_{13}(t,\mathbf{r})\rangle$ (see Eq.(17)) remains suppressed due to the dephasing of the spin PLM-coherence $\hat{S}^j_{12}(\tau+T)$ and does not lead to generation of radiation at the atomic transition $|1\rangle\leftrightarrow|3\rangle$. The solution of Eq. (13), (19) for signal field has the form:

$$\hat{b}_s(t,z)=\hat{b}_{s,0}(t-t_s-z/v_g)e^{-\alpha_sz/2}-i\frac{2\pi g_s}{v_g}\sum_{j=1}^{N}e^{-i\Delta_j(t-t_s)}\cdot \int_0^z dz'e^{-\alpha_s(z-z')/2}\hat{S}^j_{23}(\tau+T)\delta(z'-z_j), \tag{20}$$

where $\alpha_s=\alpha_{0,s}\sin^2(\frac{\theta_0}{2})$, $\alpha_{0,s}=\frac{4\pi N|g_s|^2}{v_g\Delta_{in}L}$ is the resonant absorption coefficient on the atomic transition $|2\rangle\leftrightarrow|3\rangle$, operator $\hat{b}_{s,0}(t-t_s-z/v_g)$ describes input signal field.

The first terms of the solution (20) describes the absorption of the signal pulse. The second term in signal field is determined by the initial values of atomic operators $\hat{S}^j_{23}(\tau+T)$, which, due to the initial ground atomic state, do not contribute to the excited states of signal radiation and atoms. Therefore, we will omit such terms in the field and atom operators below After absorption of the signal pulse $(t>t_s+\delta t_s)$ ($\delta t_s$ is a signal pulse duration), the excited optical coherences of the j-th atom are equal to

$$\hat{S}^j_{23}(t)=-ig_se^{-i\Delta_j(t-t_s)-\alpha_sz_j/2}\sin^2(\frac{\theta_0}{2})\tilde{b}_{s,0}(\Delta_j), \tag{21}$$

$$\hat{S}^j_{13}(t)=\frac{g_s}{2}e^{-i\Delta_j(t-t_s-T)+i\phi}\sin\theta_0\cdot e^{i\delta\mathbf{k}_{sc}\mathbf{r}_j-\alpha_sz_j/2}\tilde{b}_{s,0}(\Delta_j), \tag{22}$$

where $\delta\mathbf{k}_{sc}=\mathbf{k}_0-\mathbf{k}_1+\mathbf{k}_2$ is a wave vector of spin coherence, $\tilde{b}_{s,0}(\Delta_j)=\int_{-\infty}^{\infty}dte^{i\Delta_jt}\hat{b}_{s,0}(t)$ is a Fourier component of the input signal.

As it is seen in Eq.(22), the macroscopic optical coherence $\langle\hat{S}^j_{13}(t)\rangle$ is rephased at the moment of time $t=t_e=t_s+T$ that can cause an echo signal emission with a delay time of $T$ after the arrival of the signal pulse. The echo signal will be emitted on atomic transition $|1\rangle\leftrightarrow|3\rangle$ with carrier frequency $\omega_e=\omega_{31}$ along wave vector $\mathbf{k}_e(\omega_{31})$ when the phase matching condition is met (see also equation for $P^j_{13}$ in (11))

$$\mathbf{k}_e(\omega_{31})\cong\mathbf{k}_s+\delta\mathbf{k}_{sc}. \tag{23}$$

The application of the backward scheme providing effective echo emission proposed in the CRIB protocol [4] is possible when $\mathbf{k}_e(\omega_{31})=-k_e(\omega_{31})\mathbf{e}_z$, which can be implemented by using the following wave vectors of signal, RF and two control laser pulses $\mathbf{k}_2\uparrow\downarrow\mathbf{k}_1\uparrow\uparrow\mathbf{k}_0\uparrow\uparrow\mathbf{k}_s$ where $k_0\ll k_{1,2}$ and $k_s<k_{1,2}$. Below we consider this scheme of echo emission.

### C. Backward scheme of echo retrieval

Assuming that the phase matching condition is met, we similarly get the following equations for the optical coherence of $\hat{S}^j_{13}$ atoms and the echo signal $\hat{b}_e(t,z)$:

$$\left(\frac{\partial}{\partial t} - v_g \frac{\partial}{\partial z}\right) \hat{b}_e(z,t) = -2\pi i \sum_{j=1}^{N} g_e \hat{S}^j_{13}(t)\delta(z - z_j), \tag{24}$$

$$\frac{\partial \hat{S}^j_{13}(t)}{\partial t} = -i\Delta_j \hat{S}^j_{13}(t) - i g_e \hat{b}_e(z_j,t)\hat{S}^j_{11}(t), \tag{25}$$

where $\hat{b}_e(t,z) = e^{i\omega_e t + ik_e z}\hat{a}_e(t,z)$, $\hat{S}^j_{13}(t) = e^{i\omega_e t + ik_e z}\hat{P}^j_{13}(t)$, $g_e = E_0\langle \mathbf{d}_{13} \cdot \mathbf{e}\rangle/\hbar$ is a coupling constant of photon with atom on transition $|1\rangle \leftrightarrow |3\rangle$. In solution of Eqs. (24), (25) we take into account initial behaviour of $\langle \hat{S}^j_{13}(t)\rangle$ (22) and $\langle \hat{S}^j_{11}(t)\rangle = \cos^2(\theta_0/2)$ for the long-lived spin states. Finding atomic coherence $\hat{S}^j_{13}(t)$, using its initial state and the formal response to the emitted photon echo signal, we obtain the Heisenberg equation for this signal

$$\left(\frac{\partial}{v_g \partial t} - \frac{\partial}{\partial z}\right) \hat{b}_e(z,t) = -\frac{\alpha_e}{2}\hat{b}_e(z,t) - ie^{i\phi}\frac{g_s}{2g_e}\alpha_{0,e}\sin\theta_0 e^{-\alpha_s z/2}\hat{b}_s(t - t_s - T + z/v_g), \tag{26}$$

where $\alpha_e = \alpha_{0,e}\cos^2(\frac{\theta_0}{2})$ is the absorption coefficient on the atomic transition $|1\rangle \leftrightarrow |3\rangle$, $\alpha_{0,e} = \frac{4\pi N |g_e|^2}{v_g \Delta_{in} L}$, $g_e = E_0\langle \mathbf{d}_{13} \cdot \mathbf{e}\rangle/\hbar$ is the coupling constant of the photon-atom interaction.

Solution of (26) is

$$\hat{b}_e(z,t) = -ie^{i\phi}\frac{2(\frac{g_s}{g_e})\tan(\frac{\theta_0}{2})}{1 + |\frac{g_s}{g_e}|^2 \tan^2(\frac{\theta_0}{2})}\hat{b}_s(t - t_s - T + z/v_g)\cdot e^{\alpha_e z/2}\left[e^{-(\alpha_e+\alpha_s)z/2} - e^{-(\alpha_e+\alpha_s)L/2}\right]. \tag{27}$$

Here again we keep only the operators that describe the non-vacuum field terms.

On leaving the optically depth medium ($z = 0$, $(\alpha_e + \alpha_s)L \gg 1$) if $|\frac{g_s}{g_e}|\tan(\frac{\theta_0}{2}) = 1$ (i.e. the equality of absorption coefficients at both atomic transitions $\alpha_s = \alpha_e$), we get for the echo signal having the following solution in free space

$$\hat{b}_e(z < 0, t) = -ie^{i\phi}\hat{b}_s(t - t_s - T + z/v_g). \tag{28}$$

The solution (28) describes perfect recover of the input signal optical field. The only differences are the emission of the echo signal at a different frequency and the appearance of a constant phase shift in it, which do not change the quantum properties of the emitted photon echo, which are completely borrowed from the input signal pulse.


[1] M. Nilsson, L. Rippe, S. Kröll, R. Klieber, and D. Suter, Hole-burning techniques for isolation and study of individual hyperfine transitions in inhomogeneously broadened solids demonstrated in $Pr^{3+}$:$Y_2SiO_5$, Phys. Rev. B **70**, 214116 (2004).

[2] M. Afzelius, I. Usmani, A. Amari, B. Lauritzen, A. Walther, C. Simon, N. Sangouard, J. Minář, H. de Riedmatten, N. Gisin, and S. Kröll, Demonstration of atomic frequency comb memory for light with spin-wave storage, Phys. Rev. Lett. **104**, 040503 (2010).

[3] M. O. Scully and M. S. Zubairy, *Quantum Optics* (Cambridge University Press, 1997).

[4] S. A. Moiseev and S. Kröll, Complete reconstruction of the quantum state of a single-photon wave packet absorbed by a doppler-broadened transition, Phys. Rev. Lett. **87**, 173601 (2001).
